# Supplementary material for: RSLM: Training-Free Vector Quantization for Approximate Nearest Neighbor Search
Source: arXiv:2608.30384 source file (2026-08-31)
Supplement: Supplementary file 1 [file e2e-more-results.tex]

% delete
