# Supplementary material for: RSLM: Training-Free Vector Quantization for Approximate Nearest Neighbor Search
Source: arXiv:2608.30384 source file (2026-08-31)
Supplement: Supplementary file 2 [file res-quant-faiss.tex]

% \subsection{Residual Quantization in Faiss}

% \Teodora{here we can show the Faiss PRQ results from \url{https://g3doc.corp.google.com/experimental/users/teodoradobos/faiss_tests/g3doc/faiss_vs_astro_residual_quantization.md?cl=953314145}; this way, we show that RelApprox-Codec is a better alternative to existing residual quantization techniques}
